# Supplementary material for: Ferroelectric texture of individual barium titanate nanocrystals
Source: arXiv:2402.14502 source file (2024-07-09)
Supplement: Supplementary file 1 [file SupplInformation_nanoBTO_ferroelectric_texture_red.pdf]

# Supporting Information

## Ferroelectric texture of individual barium titanate nanocrystals


Athulya K. Muraleedharan,[†] Kevin Co,[‡] Maxime Vallet,[‡] Abdelali Zaki,[‡] Fabienne Karolak,[‡] Christine Bogicevic,[‡] Karen Perronet,[†] Brahim Dkhil,[‡] Charles Paillard,[‡,¶] Céline Fiorini-Debuisschert,[§] and François Treussart[*,†]

†*Université Paris-Saclay, ENS Paris-Saclay, CNRS, CentraleSupélec, LuMIn, 91190 Gif-sur-Yvette, France*

‡*Université Paris-Saclay, CentraleSupélec, CNRS, Laboratoire SPMS, 91190 Gif-sur-Yvette, France*

¶*Smart Ferroic Materials, Institute for Nanoscience & Engineering and Department of Physics, University of Arkansas, Fayetteville 72701 Arkansas, United States*

§*Université Paris-Saclay, CEA, CNRS, SPEC, 91191 Gif-sur-Yvette, France*

E-mail: francois.treussart@ens-paris-saclay.fr

# 1. Supporting text

## S1. Basic principles of piezoresponse force microscopy

In piezoresponse force microscopy, a conducting tip to which an oscillating voltage $V_{\mathrm{tip}} = V_{\mathrm{AC}} \cos(2\pi f_{\mathrm{d}} t)$ is applied is brought into contact with the grounded sample, causing a surface deformation due to the inverse piezoelectric effect. From the resulting oscillatory response of the material, the device extracts the first harmonic component of the deflection of the AFM tip $D = A \cos(2\pi f_{\mathrm{d}} t + \varphi)$, where $A$ is the deflection amplitude to which the magnitude of the local piezoresponse displacement $u$ is proportional, and $\varphi$ is the phase change between the driving voltage and the voltage-induced deformation that depends on the local polarization of the material.[1] The deflection is measured using a laser beam that is reflected off the cantilever onto a position-sensitive quadrant photodiode. PFM cantilever undergoes two types of deformations: vertical deformation due to the out-of-plane/vertical domains (VPFM) or/and torsion due to the shear deformation induced by the in-plane/lateral domains (LPFM). PFM measurement consists of mapping the piezoresponse amplitude and phase signals in both the VPFM and LPFM modes. The electromechanical response of a ferroelectric material of arbitrary crystallographic orientation to an applied voltage is a vector having three independent components of piezoresponse: one VPFM measurement and two LPFM measurements in two independent directions. The third component of the displacement vector can be determined by imaging the sample region of the sample after a 90° rotation around the $z$ axis. When all three components of the piezoresponse are acquired, it is possible to reconstruct a 3-dimensional local electromechanical mixed response vector map. This approach is called a vector PFM, described in details in Kalinin *et al.*[2]

## S2. Phase field simulations: analytical expressions of the contributions to the free energy volume density

In this section, $(x, y, z)$-coordinates are attached to the material. Unless otherwise specified we use in an indiscriminate manner the letter $(x, y, z)$ or number (1,2,3) indices. Below are the analytical expressions of the different terms of Helmoltz free energy density $f_{\mathrm{H}} \equiv f_{\mathrm{bulk}} + f_{\nabla P} + f_{\mathrm{elastic}} + f_{\mathrm{electrostr}} + f_{\mathrm{elec}}$, as stated in refs.[3,4]

$$
\begin{aligned}
f_{\mathrm{bulk}} &= \alpha_1(P_x^2+P_y^2+P_z^2)+\alpha_{11}^{(e)}(P_x^4+P_y^4+P_z^4)\\
&+ \alpha_{12}^{(e)}(P_x^2P_y^2+P_x^2P_z^2+P_y^2P_z^2)+\alpha_{111}(P_x^6+P_y^6+P_z^6)\\
&+ \alpha_{112}(P_x^4(P_y^2+P_z^2)+P_y^4(P_x^2+P_z^2)+P_z^4(P_y^2+P_x^2))\\
&+ \alpha_{123}P_x^2P_y^2P_z^2
\end{aligned} \tag{1}
$$

The gradient energy density, $f_{\nabla P}$, contains the first-order Lifshitz invariant

$$
\begin{aligned}
f_{\nabla P} &= \frac{G_{11}}{2}\left(\frac{\partial P_x}{\partial x}+\frac{\partial P_y}{\partial y}+\frac{\partial P_z}{\partial z}\right)\\
&+ G_{14}\left(\frac{\partial P_x}{\partial x}\frac{\partial P_y}{\partial y}+\frac{\partial P_x}{\partial x}\frac{\partial P_z}{\partial z}+\frac{\partial P_z}{\partial z}\frac{\partial P_y}{\partial y}\right)\\
&+ \frac{G_{44}}{2}\left(\left(\frac{\partial P_x}{\partial y}\right)^2+\left(\frac{\partial P_y}{\partial x}\right)^2+\left(\frac{\partial P_x}{\partial z}\right)^2+\left(\frac{\partial P_z}{\partial x}\right)^2+\left(\frac{\partial P_z}{\partial y}\right)^2+\left(\frac{\partial P_y}{\partial z}\right)^2\right)
\end{aligned} \tag{2}
$$

Contributions to the elastic volume energy density comes from the strain tensor $\varepsilon_{\alpha\beta}$ defined in terms of the local displacement field $\boldsymbol{u}(\boldsymbol{r})$:

$$
\varepsilon_{\alpha\beta} = \frac{1}{2}\left(\frac{\partial u_\alpha}{\partial \beta}+\frac{\partial u_\beta}{\partial \alpha}\right), \alpha, \beta = x, y \text{ or } z. \tag{3}
$$

The elastic energy density is then written in terms of the elastic constants $C_{ij}$, and using

Voigt's notation ($\varepsilon_1 = \varepsilon_{11}, \varepsilon_2 = \varepsilon_{22}, \varepsilon_3 = \varepsilon_{33}, \varepsilon_4 = 2\varepsilon_{23}, \varepsilon_5 = 2\varepsilon_{13}$, and $\varepsilon_6 = 2\varepsilon_{12}$) as

$$\begin{aligned} f_{\text{elastic}} &= \frac{1}{2}C_{11}\left(\varepsilon_1^2 + \varepsilon_2^2 + \varepsilon_3^2\right) \\ &+ C_{12}\left(\varepsilon_1\varepsilon_2 + \varepsilon_1\varepsilon_3 + \varepsilon_2\varepsilon_3\right) \\ &+ \frac{1}{2}C_{44}\left(\varepsilon_4^2 + \varepsilon_5^2 + \varepsilon_6^2\right) \end{aligned} \tag{4}$$

The electrostrain energy density is written

$$\begin{aligned} f_{\text{electrostr}} &= -q_{11}\left[\varepsilon_1 P_x^2 + \varepsilon_2 P_y^2 + \varepsilon_3 P_z^2\right] \\ &- q_{12}\left[\varepsilon_1\left(P_y^2 + P_z^2\right) + \varepsilon_2\left(P_x^2 + P_z^2\right) + \varepsilon_3\left(P_y^2 + P_x^2\right)\right] \\ &- q_{44}\left[\varepsilon_6 P_x P_y + \varepsilon_5 P_x P_z + \varepsilon_4 P_y P_z\right] \end{aligned} \tag{5}$$

At last, the electric energy $f_{\text{elec}} = -\boldsymbol{E}(\boldsymbol{r}).\boldsymbol{P}(\boldsymbol{r})$, where $\boldsymbol{E}(r)$ is the electric field obtained from solving the Poisson equation.

All numerical coefficients involved here were taken from Ref.[3]

# 2. Supporting data

## 2.1. BTO sample additional characterizations

### BTO nanocrystals morphology and strain

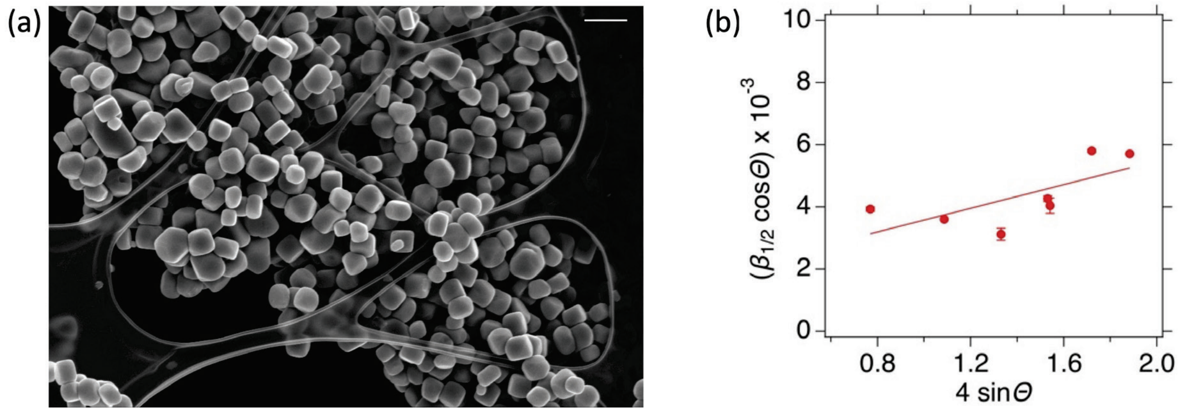


Figure S1: **Morphology and strain of as-produced BTO nanocrystals**. (a) SEM image of BTO NC powder deposited on a carbon layer, showing mostly parallelepipedic/cubic shape particles. SEM model: XL30S FEG from FEI/Philips (The Netherlands). Scale bar: 400 nm. (b) Estimate of the strain from the diffractogram Figure 1a, using Williamson-Hall method. The experimental points are the diffraction peaks positions, and the solid line a fit according to equation (6).

Figure S1a shows a "large" SEM field of view of the as-produced BTO nanocrystal powder. This powder was the starting material to prepare the BTO NCs aqueous suspension from which individual particles were isolated. We also estimate the strain from Figure 1a diffractogram of this powder using the Williamson-Hall equation for a Cauchy peak shape:

$$\beta_{1/2}\cos\theta = \frac{K\lambda}{D} + 4e\sin\theta, \tag{6}$$

where $\beta_{1/2}$ is the full-width at half-maximum of each diffraction peak, $\lambda$ is the X-ray radiation wavelength (here $\lambda = 1.5418$ Å, $D$ and $e$ the grain size and inhomogeneous strain, respectively, and $K$ is a NC form factor that we took equal to 1. Figure S1b displays the experimental points for each diffraction peak and the linear fit according to equation 6, leading

to a strain $e = 0.19 \pm 0.04\%$ and a crystallographic grain size $D = 81$ nm.

**HR-STEM Image**

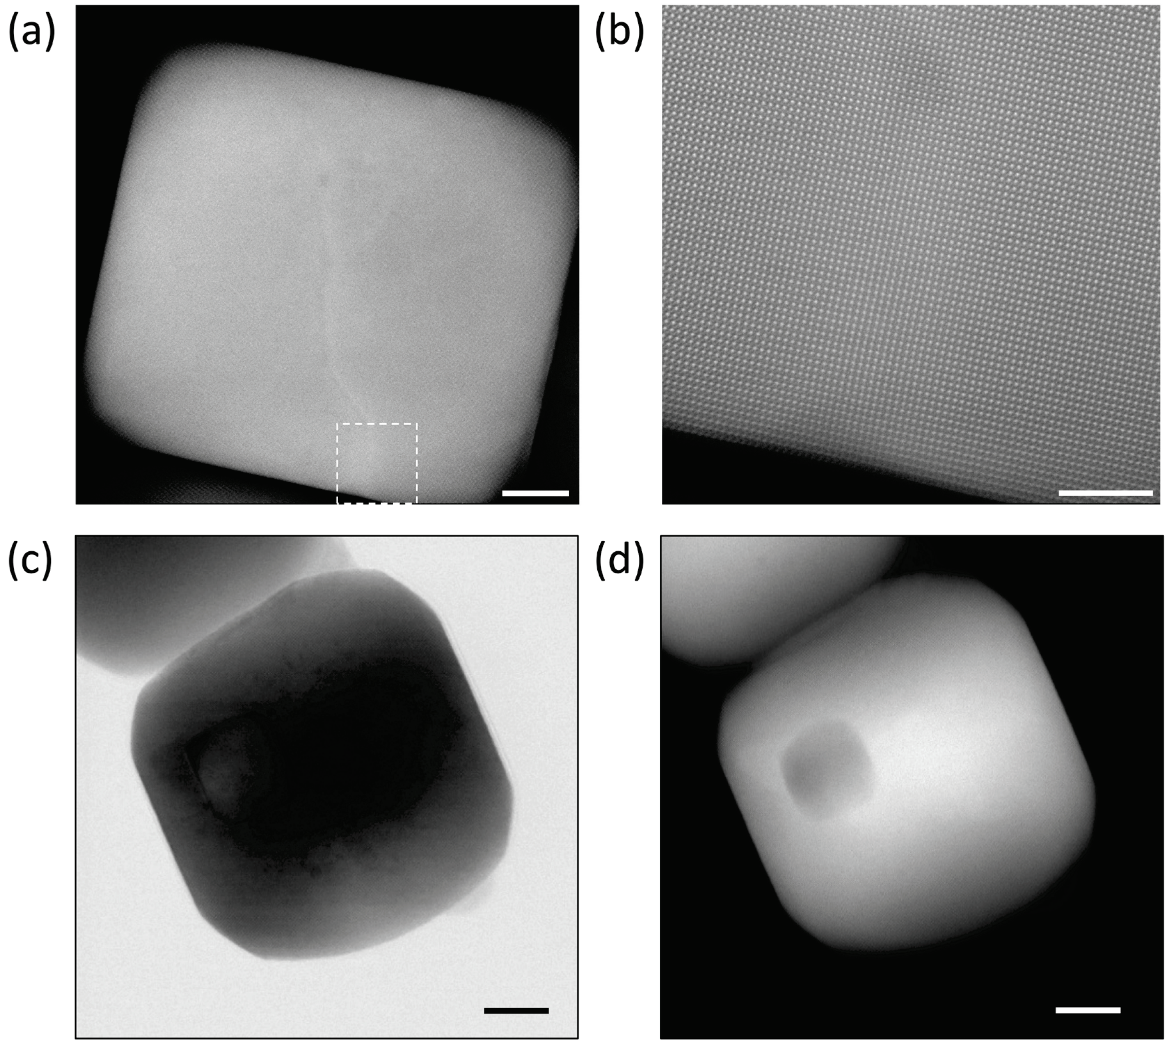


Figure S 2: **Additional STEM images of single BTO nanocrystals**. (a) HAADF STEM image of one BTO NC. Scale bar: 20 nm. (b) Atomic resolution image of the region delineated by the dashed line square in (a), with no evidence of a thin layer of cubic crystalline symmetry at the NC surface. Scale bar: 5 nm. (c) Bright-field and (d) HAADF images of a different, much rounder NC, showing a $\approx 20$ nm-sized pore defect within the particle. Scale bars: 20 nm.

Figure S2 shows HR-STEM images of an individual BTO NC oriented relative to the electron beam to yield atomic column resolution (Figure S2b). We do not observe that the NC has any layer of different crystallographic symmetry than the one at its center. Note that the line crossing the NC from top to bottom on Figure S2a may be either a structural defect or an in-plane domain wall.

### Evidence of a phase transition from temperature dependence Raman spectroscopy of BTO nanopowder

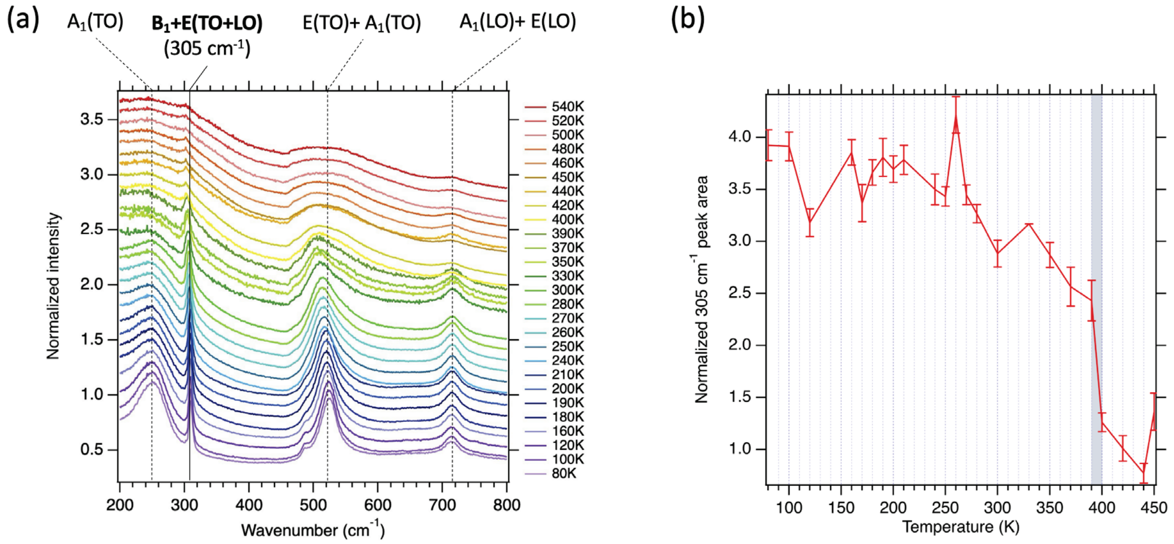


Figure S3: **Temperature dependence of BTO Raman spectrum and Curie temperature estimate**. (a) Raman spectrum of BTO nanopowder at temperatures varying from 80 K to 540 K. In the tetragonal phase (space group P4mm) BTO symmetry belongs to the point group $C^1_{4v}$ which irreducible representation is $\Gamma^{\text{optic}}_{C_{4v}} = 3(A_1 + E) + E + B_1$. Due to long-range electrostatic forces, the $A_1$ and $E$ modes are further divided into transverse and longitudinal optical modes (LO and TO, respectively[5]). On top of the graph, we identified by their group nomenclature a series of four groups of spectrally not-all-resolved peaks. All spectra were normalized to the $\approx 250$ cm$^{-1}$ peak intensity (to account for temperature depopulation), and the spectra were shifted vertically for clarity. (b) Area of the $\approx 305$ cm$^{-1}$ normalized peak versus temperature. The shaded zone indicates the range of temperature in which the peak area change most, and from which we infer a phase transition Curie temperature of $395 \pm 2$ K.

### Characterization of BTO nanocrystals bound to the substrate

The NC are attached to the numbered grid with a thin layer of PEDOT:PSS conductive polymer. A layer thickness of $\approx$ 45 nm was measured by AFM, as shown on Figure S4a,b, after having removed a tape that had been placed on an edge of the substrate before spin-coating PEDOT:PSS. Similarly, we estimated how much a NC sinks into the PEDOT:PSS before its annealing, by measuring the depth of the hole that remains in the event of the PFM tip drags the NC (Figure S4c,d). We estimate this depth to be $\approx$ 30 nm. The heightened contour encircling the hole is likely to be the concave meniscus that holds the particle, confirming the wetting of the BTO by PEDOT:PSS.

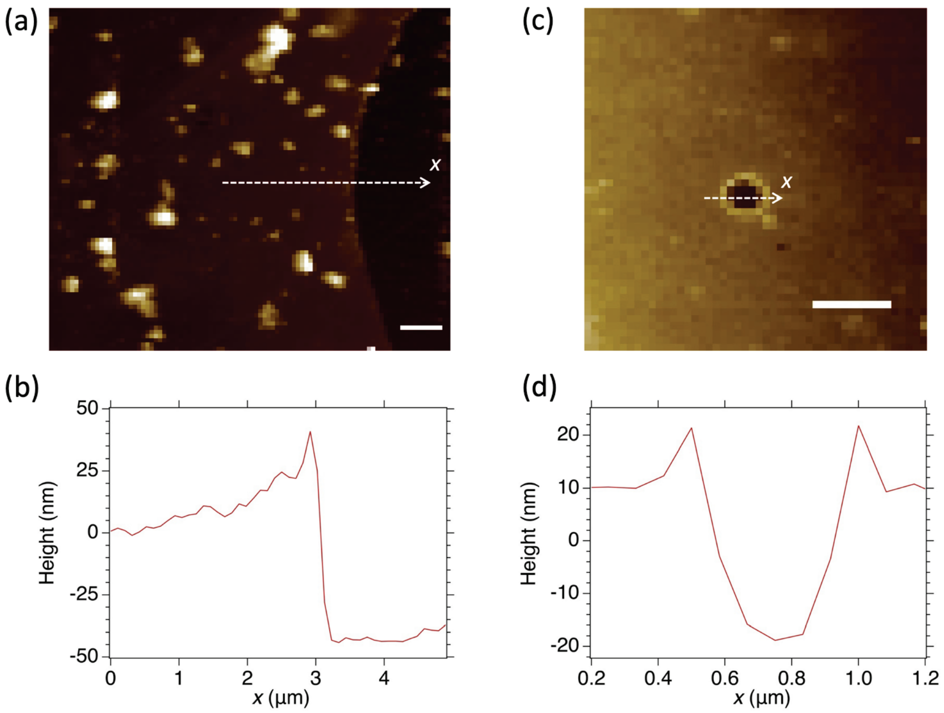


Figure S4: **PEDOT:PSS layer thickness and depth of penetration of NC in the layer**. (a) PEDOT:PSS layer near an edge of the substrate after tape removal. (b) Height profile along the dashed white line in panel (a). (c) Hole in the PEDOT:PSS layer after a NC was dragged by the PFM tip during scanning. (d) Height cross-section along the dashed line of panel (c) showing that the particle was immersed partially in the polymer layer. All scale bars: 1 $\mu$m.

The single NCs that we studied by PFM were first identified using SEM and their po-

sitions in the numbered gold grid, as shown on Figure S5a, allowed to retrieve them in PFM.

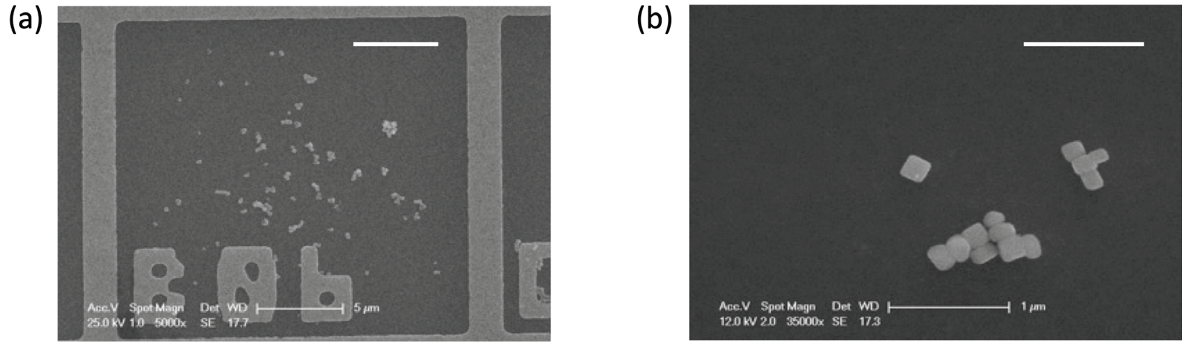


Figure S5: **BTO nanocrystals bound to the numbered gold-made grid**. (a) Large field of view that allows one to read the grid number (here B06). Scale bar: 5 $\mu$m. (b) Smaller field of view with an isolated NC candidate in the middle. Scale bar: 1 $\mu$m.

For the PFM study, we considered only isolated NCs of close to cubic shape, such as the one in the middle of Figure S5b. Figure S6 shows the size and shape distributions of the isolated NCs subsequently studied by PFM.

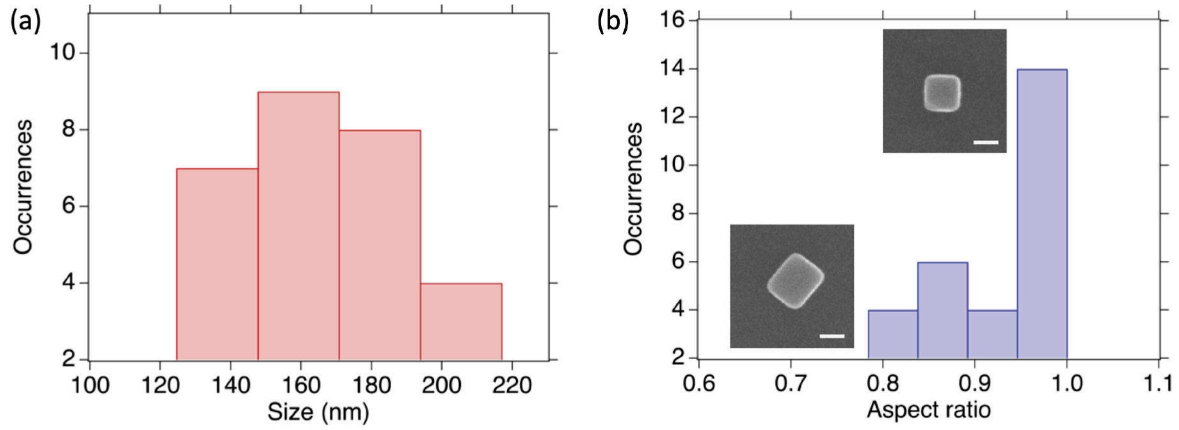


Figure S6: **Size distribution and morphology of the individual BTO nanocrystals spincoated on ITO-coated coverslip**. (a) Distribution of NCs size (defined as the mean value of the side lengths), with an average and standard deviation of $160 \pm 28$ nm. (b) Aspect ratio of the particles (defined as the size of the short side on the one of the long side), revealing a majority of particles with ratio 1, which indicates a close-to-cubic shape. Inset: SEM images of two single NCs with aspect ratios 1 and 0.8. Scale bar: 100 nm.

## 2.2. Evidence of non-electromechanical effects and use of electrostatic blind spot setting to suppress them

We evidenced the existence of non-electromechanical effects in PFM measurements and demonstrated their suppression when the laser spot used to measure the cantilever deflection is placed at an electrostatic blind spot (ESBS) position. This approach was first described in Killgore *et al.*[6]

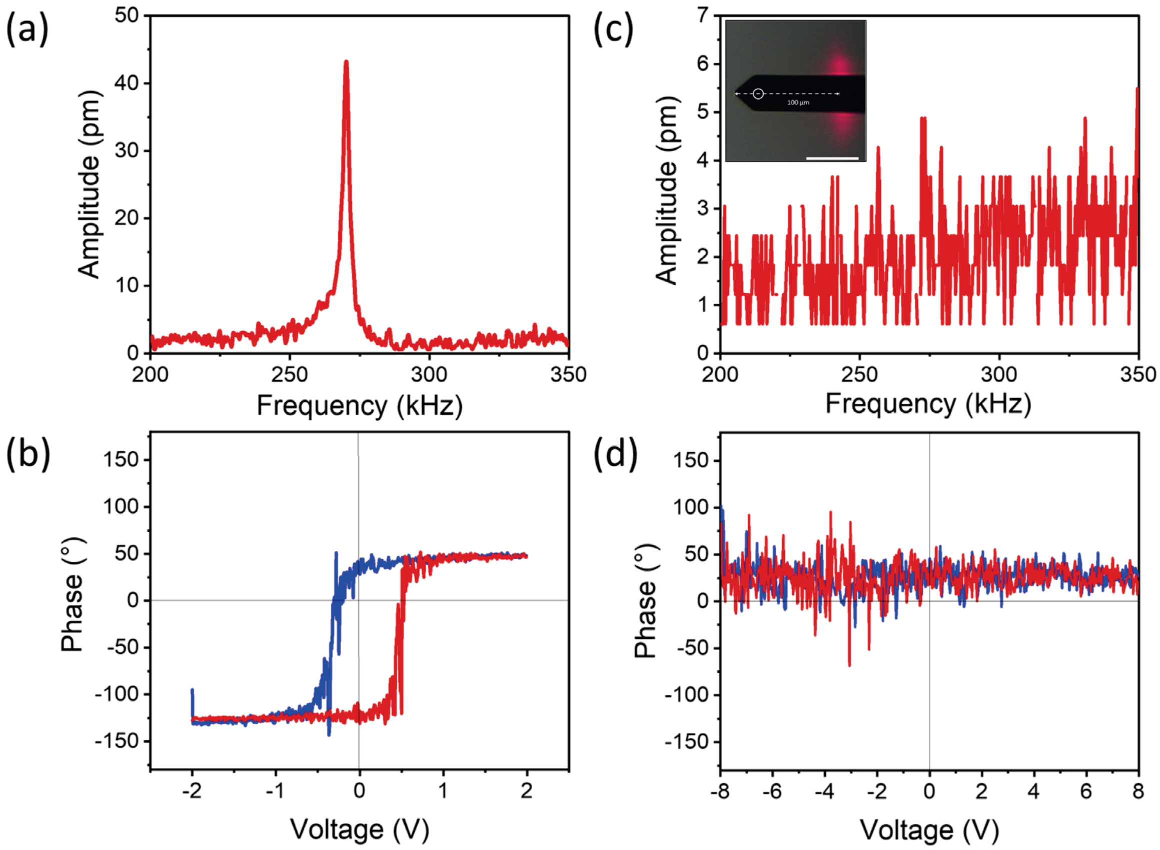


Figure S7: **PFM artifacts and their suppression by finding the ESBS position**. (a,b) When the deflection laser spot is positioned above the tip at the extremity of the cantilever, it induces a contact resonance on ITO in the 220-280 kHz range (a) and an hysteresis loop when ramping a DC bias between +2 V and -2 V (b). (c,d) By moving the laser spot away from the cantilever extremity to the ESBS position, the contact resonance can be suppressed (c) as well as the hysteresis loop (d). Inset of panel (c): picture of ESBS position of the red laser on the cantilever (length $L = 225$ $\mu$m) located at 100 $\mu$m from the cantilever tip (corresponding to $0.45L$). The conventional laser position is indicated by the white circle. Scale bar: 50 $\mu$m.

We first confirmed non-electromechanical effects leading to a PFM signal on an ITO coated substrate alone, with no ferroelectric material deposited on it. These effects were observed through different signatures that were also useful to determine ESBS position by suppressing them in situations where they should not exist, typically on non-ferroelectric materials like in our case the ITO layer. The artifacts observed included the presence of a cantilever contact resonance (Supporting Figure S7a), or a hysteresis loop (Figure S7b), or of a PFM contrast in freshly "written" regions, when the deflection laser spot was adjusted at the extremity of the cantilever, as conventionally done in atomic force microscopy.

As we moved the deflection laser spot further from the cantilever extremity, as shown on the inset picture of Figure S7c, we managed to find a position, the ESBS position, for which the contact resonance disappeared (Figure S7c) and the hysteresis cycle flattened (Figure S7d), removing the previous artifacts.

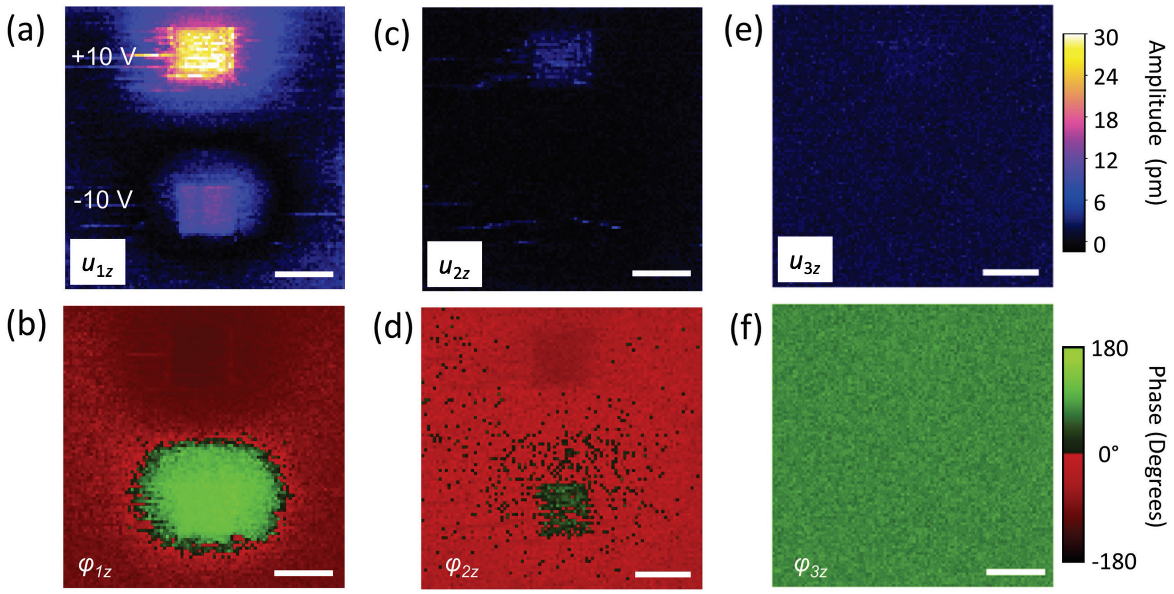


Figure S8: **Suppression of electrostatic cross-talk after adjusting AFM laser spot at ESBS location** (a,b) PFM displacement amplitude and phase maps after writing on ITO with +10 V and -10 V with the laser spot positioned at the cantilever tip. (c,d) Same region with the laser positioned halfway between the ESBS position and the tip. (e,f) Amplitude and phase images of the same region with laser at ESBS positioned approximately 100 $\mu$m away from the cantilever tip showing absence of contrast in amplitude and phase. Scale bar: 1 $\mu$m.

As mentioned, another type of electrostatic artifact could be detected in PFM phase and amplitude images of ITO surface after having written on a square of 1 $\mu$m side with +10 and -10 V potentials. Figure S8a,b shows PFM images with the deflection laser positioned at the extremity of the cantilever just above the tip. Figure S8c,d shows the same region when the laser was positioned between the tip and the ESBS position, showing a decrease in contrast in phase and amplitude signals. Finally, Figure S8e,f shows PFM amplitude and phase images of the same region when we placed the laser at ESBS position (identified by the disappearance of the contact resonance, like in Figure S7c). The absence of phase and amplitude contrasts confirms the suppression of electrostatic parasitic effects in the PFM signal.

## 2.3. Lateral PFM resonance curve of a cantilever

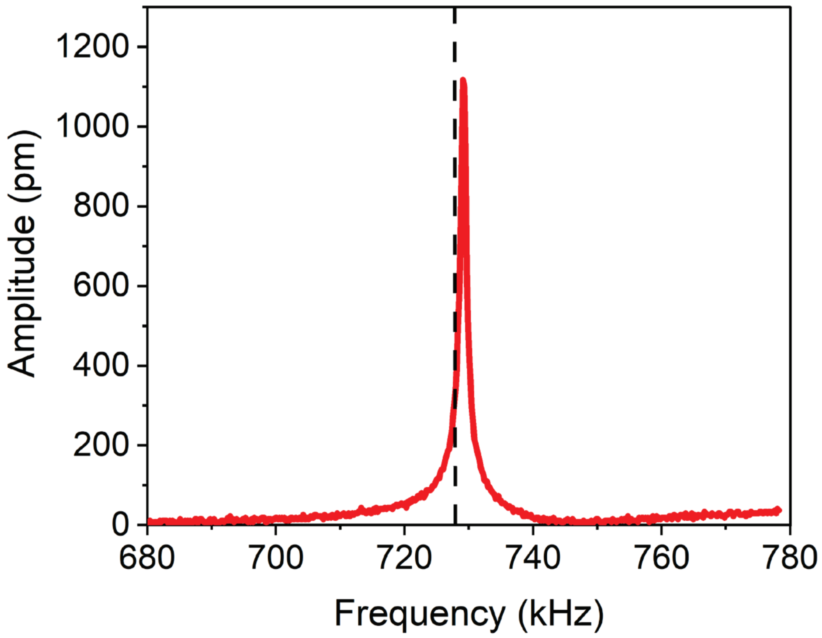


Figure S 9: **In-plane resonance curve at 730 kHz at 1.5 V drive voltage**. PFM imaging was done near the resonance peak at 727.8 kHz, indicated by the black dashed line.

## 2.4. Lateral and vertical PFM measurements on a reference sample with domains that can be oriented either in-plane or out-of-plane

We checked that the LPFM and VPFM protocols used for the characterization of nanoBTO piezoforce response (involving in particular the laser spot placed at the ESBS position), yielded the expected signals on a known sample (periodically poled lithium niobate rod), as shown on Figure S10 and Figure S11.

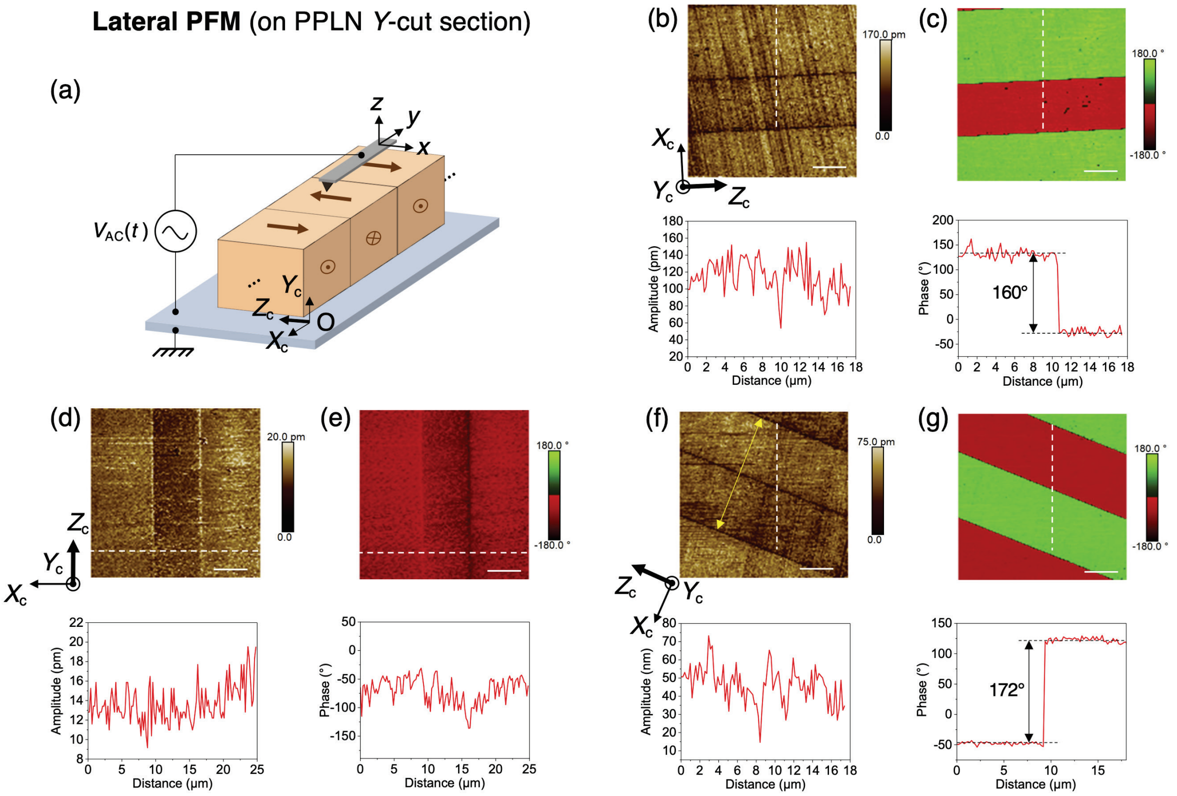


Figure S 10: **LPFM response of a $Y_c$-cut periodically poled (along $Z_c$) lithium niobate rod (PPLN)**. (a) Experimental configuration for LPFM measurement on the PPLN rod. (b) LPFM amplitude scan (top) of the sample oriented like in (a), with its poling axis $Z_c$ approximately parallel to the scanning $x$ axis. The section of the amplitude along the dashed white line is shown at the bottom. Note the decrease of amplitude at the domain wall, as expected. (c) Phase scan (top) acquired at the same time as the amplitude, showing in-plane domains of opposite $x$-projected polarizations, according to the phase difference (bottom) close to 180°.(d)-(e) Amplitude and phase scans when we orient the PPLN rod so that we scan the tip in the $(X_c, Z_c)$ plane and perpendicular to $Z_c$ axis.

Figure S 10 *(caption continues)*: The LPFM amplitude is reduced by one order of magnitude compared to (b), and the phase does not vary between domains, which is consistent with a polarization oriented solely along $Z_c$. Sections of the amplitude and phase along the dashed lines displayed in (d)-(e) are displayed at the bottom. (f)-(g) LPFM scans of the PPLN rod for an arbitrary orientation of the sample displaying amplitude values intermediate between (b) and (d) measurements. Sections of the amplitude and phase along the dashed lines displayed in (f)-(g) are displayed at the bottom. In (f) the double arrow yellow line indicates a period of the poling, which is measured at 17.6 $\mu$m. The LPFM were recorded with an AC amplitude of 2 V. The contact resonance frequency was 816.3 kHz for all measurements. (b)-(e) were performed at a driving frequency of 817.3 kHz, while for (f)-(g), the driving frequency was 815.3 kHz. All scale bars: 5 $\mu$m. The sample was cut by Prof. Mathieu Chauvet (Femto-ST, Besançon, France) from a PPLN wafer (poling axis: $Z_c$), using a precision saw, leading to a roughness $Ra \approx 5$ nm on the $Y_c$-surface. The sample dimensions are 515 $\mu$m along the crystallographic axis $Z_c$, 400 $\mu$m along $Y_c$ and 20 mm along $X_c$. One of its $Y_c$-cut face was put in contact with the grounded conductive substrate, as shown in (a), and it was further maintained by non-conductive tape. Note that the domain widths along $X_c$ are not represented at scale on (a).

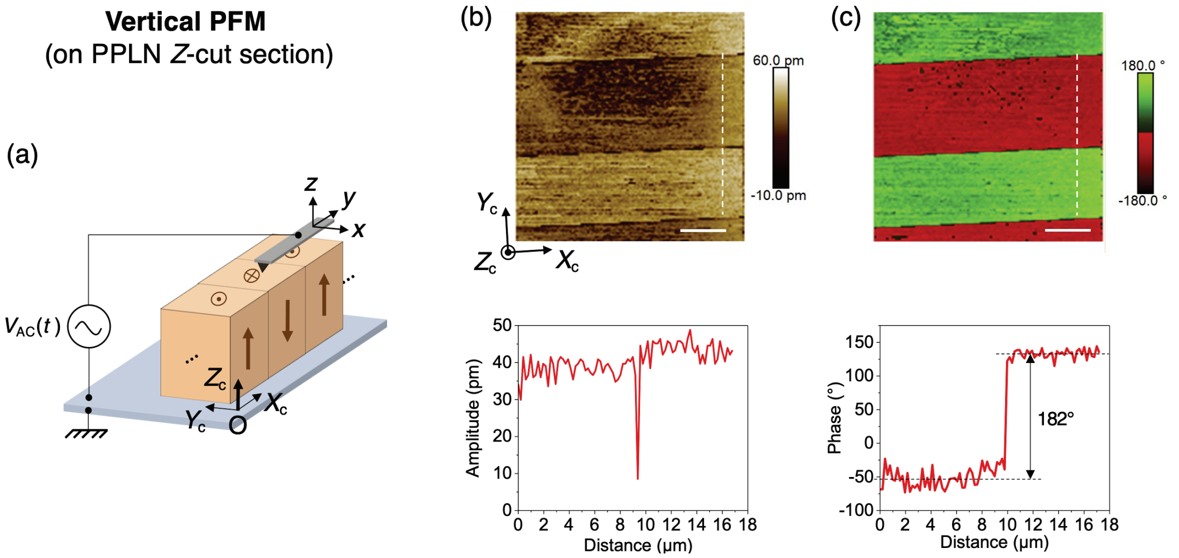


Figure S 11: **VPFM response of a $Z_c$-cut periodically poled (along $Z_c$) lithium niobate rod.** (a) Experimental configuration for VPFM measurement on the PPLN rod $Z_c$ facet (domain width not represented at scale). (b) VPFM amplitude scan (top) of the sample oriented like in (a), with its poling axis $Z_c$ vertical, out of the scanning plane $(x, y)$. The section of the amplitude along the dashed white line is shown at the bottom. Note the decrease of amplitude at the domain wall, as expected. (c) Phase scan (top) acquired at the same time as the amplitude, showing out-of-plane domains of opposite $z$-projected polarizations, according to the phase difference (bottom) very close to 180°. All scale bars: 5 $\mu$m.

## 2.5. Lateral PFM mapping of three additional BTO NCs

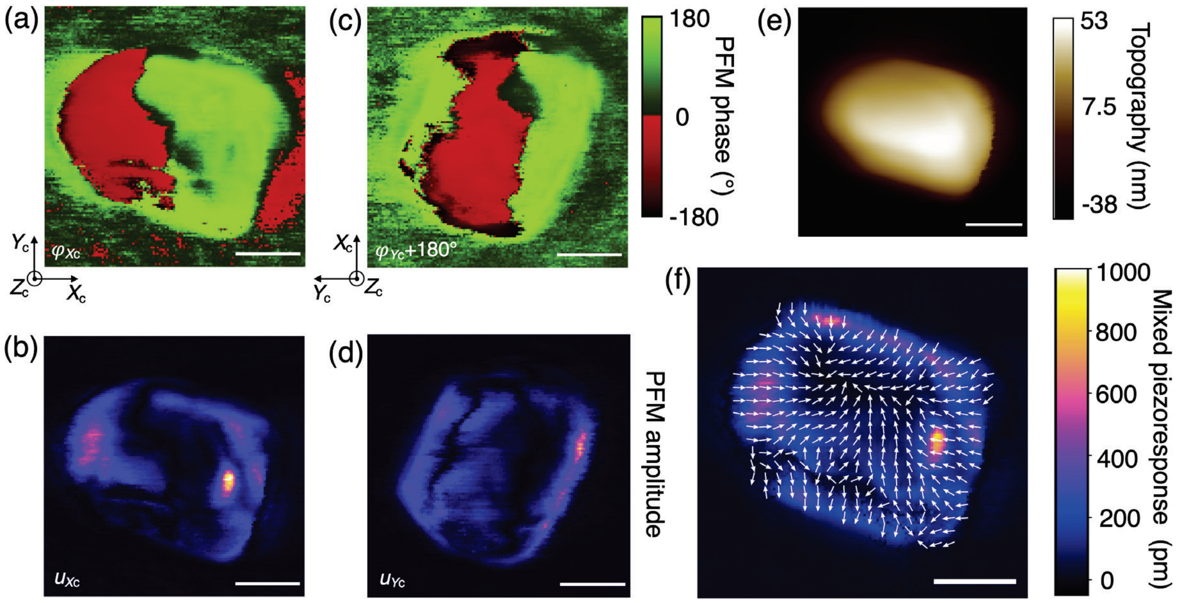


Figure S 12: **Lateral piezoresponse displacement mapping on the single BTO NC#2**. (a,b) Lateral piezoresponse phase $\varphi_x$ and amplitude $u_x$ along $x$- axis. (c,d) Lateral piezoresponse phase $\varphi_y$ and amplitude $u_y$ along the $y$- axis (sample rotated counterclockwise). (e) Topography image of the particle. (f) Mixed lateral piezoresponse field $\boldsymbol{u}^{\mathrm{m}}\,[u_{X_c}\cos(\varphi_{X_c}-\varphi_{\mathrm{offset}}), u_{Y_c}\cos(\varphi_{Y_c}-\varphi_{\mathrm{offset}})]$, with $\varphi_{\mathrm{offset}} = 34°$, displayed by superimposed norm maps (color code) and direction (array of fixed-length arrows at nodes of a 7.8 nm pitch grid). Scale bars (all scans): 50 nm. The NC in-plane sizes, further inferred from SEM image are about: 90 nm $\times$ 120 nm.

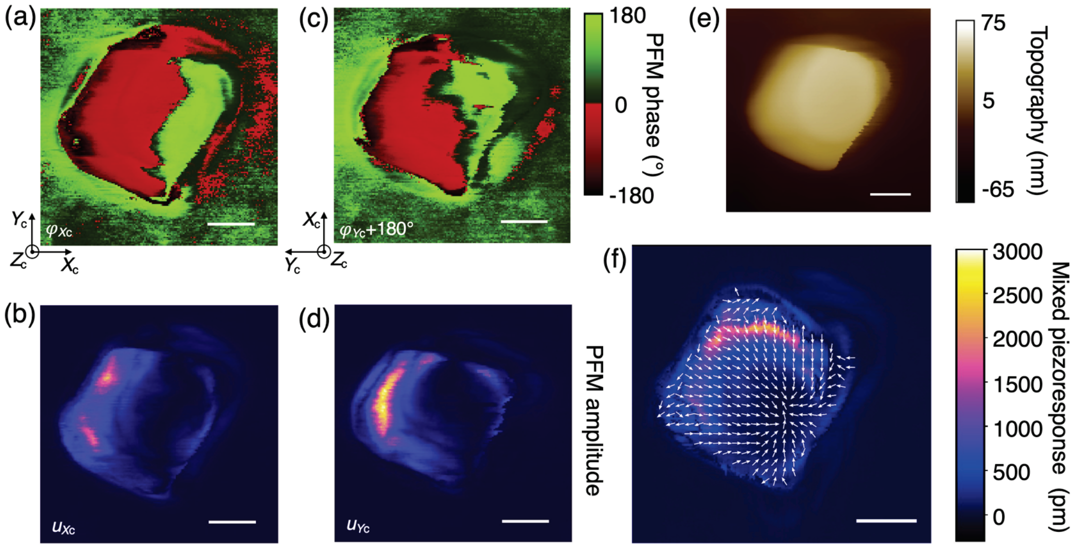


Figure S13: **Lateral piezoresponse displacement mapping on the single BTO NC#3**. (a,b) Lateral piezoresponse phase $\varphi_x$ and amplitude $u_x$ along $x$- axis. (c,d) Lateral piezoresponse phase $\varphi_y$ and amplitude $u_y$ along $y$- axis (Sample rotated counterclockwise. (e) Topography image of the particle. (f) Mixed lateral piezoresponse field $\boldsymbol{u}^{\mathrm{m}}$ $[u_{X_c}\cos(\varphi_{X_c} - \varphi_{\mathrm{offset}}), u_{Y_c}\cos(\varphi_{Y_c} - \varphi_{\mathrm{offset}})]$ with $\varphi_{\mathrm{offset}} = 20°$, displayed by superimposed maps of norm (color code) and direction (array of fixed-length arrows at nodes of a 7.8 nm pitch grid). Scale bars (all scans): 50 nm. The NC in-plane sizes, further inferred from SEM image are about: 125 nm $\times$ 130 nm.

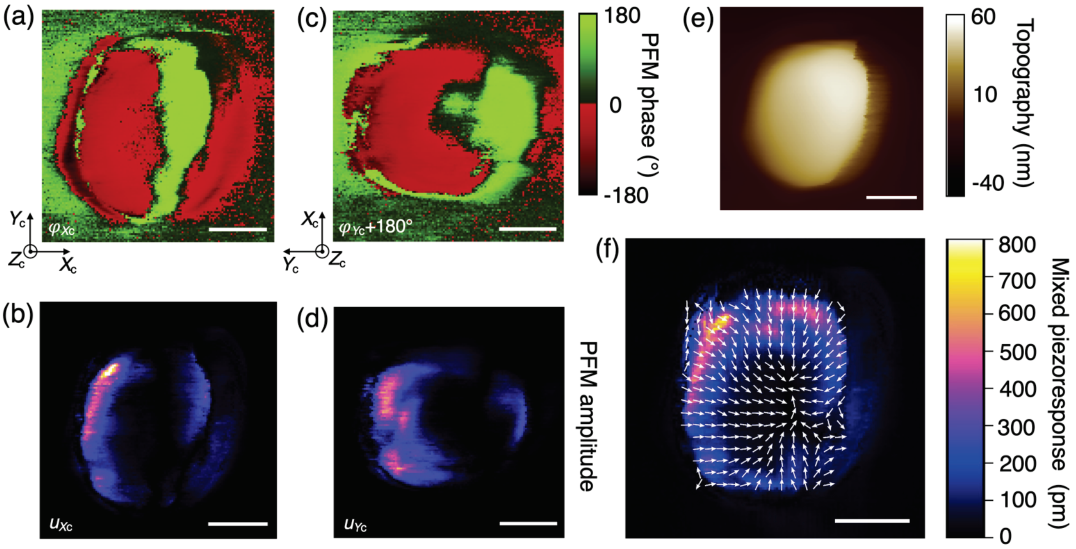


Figure S14: **Lateral piezoresponse displacement mapping on the single BTO NC#4**. (a,b) Lateral piezoresponse phase $\varphi_x$ and amplitude $u_x$ along $x$- axis. (c,d) Lateral piezoresponse phase $\varphi_y$ and amplitude $u_y$ along $y$- axis (Sample rotated counterclockwise. (e) Topography image of the particle. (f) Mixed lateral piezoresponse field $\boldsymbol{u}^{\mathrm{m}}$ $[u_{X_c}\cos(\varphi_{X_c} - \varphi_{\mathrm{offset}}), u_{Y_c}\cos(\varphi_{Y_c} - \varphi_{\mathrm{offset}}))]$, with $\varphi_{\mathrm{offset}} = 15°$, displayed by superimposed maps of norm (color code) and direction (array of fixed-length arrows at nodes of a 7.8 nm pitch grid). Scale bars (all scans): 50 nm. The NC in-plane sizes, further inferred from SEM image are about: 105 nm $\times$ 140 nm.

## 2.6. Additional data on phase field simulations

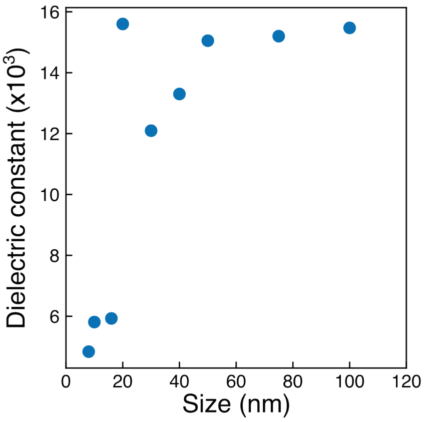


Figure S15: **Dielectric constant as a function of the nanocrystal size**. The dielectric constant $\varepsilon_r$ was inferred from phase field simulation and is considered as a probe of the ferroelectric domain structure and its response to an applied electric field. The sharp increase of $\varepsilon_r$ at the size of 20 nm is likely to reflect the transition from single to multiple polarization domains.

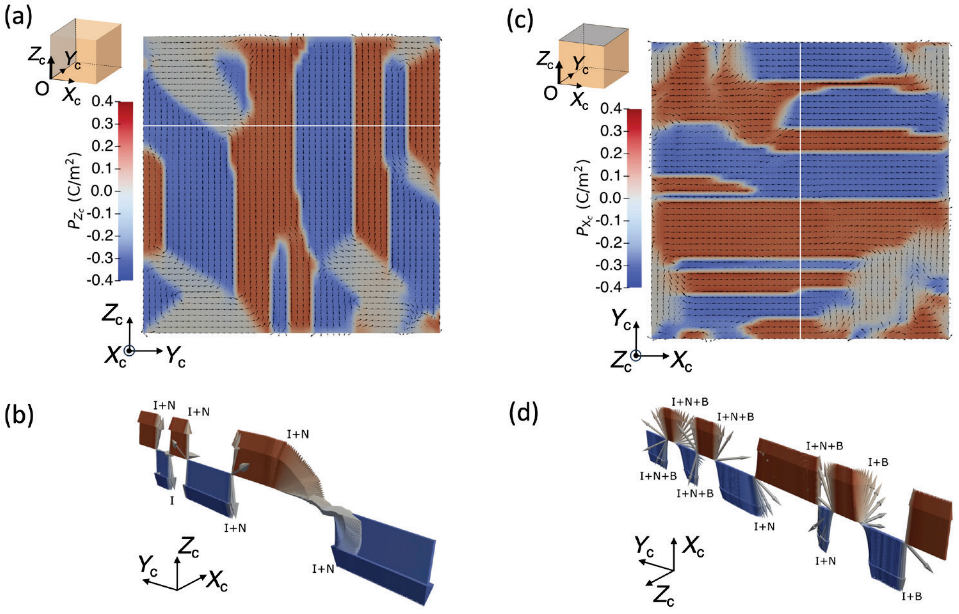


Figure S16: **Distribution of polarization in facets parallel or orthogonal to the polar axis, and illustration of the type of domain walls they host**. (a) The distribution of polarization on facet ($Y_cOZ_c$) at $X_c = 0$ nm shows the presence of $\pm Z_c$-oriented domains with $\pm Y_c$ domains near the surfaces. (b) Three-dimensional representation of the direction of the polarization vector $\boldsymbol{P}/|\boldsymbol{P}|$ showing the partial Néel nature of the walls of the predominantly Ising domain along the line ($X_c = 0$ nm$, Y_c, Z_c = -71$ nm). (c) The distribution of polarization on the $Z_c = 100$ nm top facet shows a predominantly $\pm X_c$ oriented polar domain (red and blue) with some $\pm Y_c$ oriented domains (gray). (d) Three-dimensional representation of the direction of the polarization vector showing that the domain walls along the line ($X_c = 50$ nm$, Y_c, Z_c = 100$ nm) present the partial Néel or/and Bloch character of the main Ising domain walls.

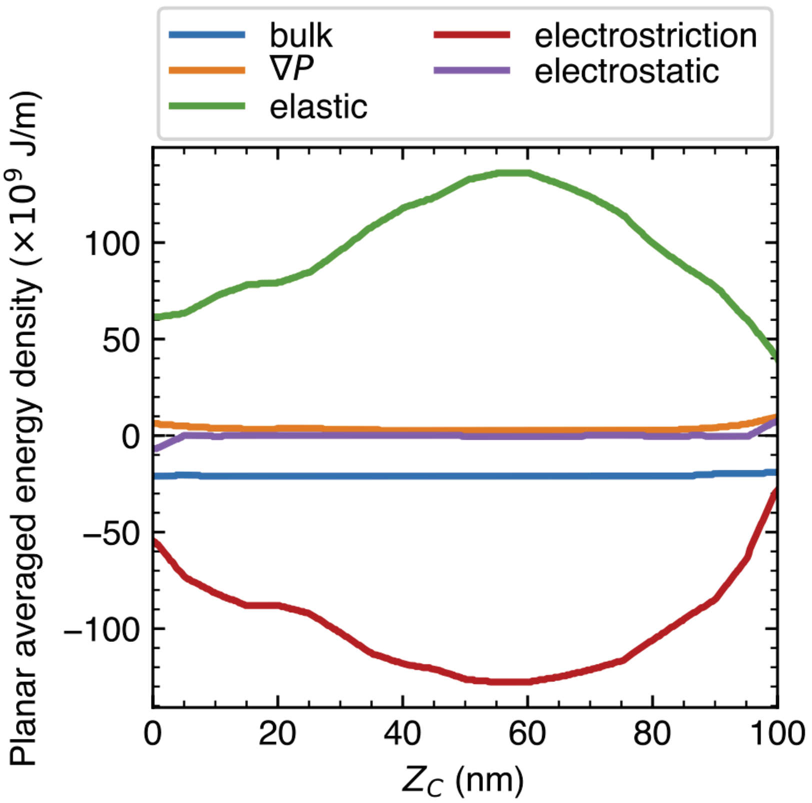


Figure S17: **Distribution of the different components of the energy density across a nanocrystal**. Planar averaged energy density contributions showing the bulk energy density (blue), the gradient of polarization energy density (orange), the elastic energy density (green), the electrostatic energy density (purple) and electrostrictive energy density (red). Energy densities are averaged in planes perpendicular to the main polar axis $Z_c$.

# References


1. Kalinin, S. V.; Rodriguez, B. J.; Jesse, S.; Karapetian, E.; Mirman, B.; Eliseev, E. A.; Morozovska, A. N. Nanoscale Electromechanics of Ferroelectric and Biological Systems: A New Dimension in Scanning Probe Microscopy. *Annual Review of Materials Research* **2007**, *37*, 189–238.

2. Kalinin, S. V.; Rodriguez, B. J.; Jesse, S.; Shin, J.; Baddorf, A. P.; Gupta, P.; Jain, H.; Williams, D. B.; Gruverman, A. Vector Piezoresponse Force Microscopy. *Microscopy and*

*Microanalysis* **2006**, *12*, 206–220.

3. Hlinka, J.; Marton, P. Phenomenological model of a 90° domain wall in $BaTiO_3$-type ferroelectrics. *Physical Review B* **2006**, *74*, 104104.

4. Mangeri, J.; Espinal, Y.; Jokisaari, A.; Pamir Alpay, S.; Nakhmanson, S.; Heinonen, O. Topological phase transformations and intrinsic size effects in ferroelectric nanoparticles. *Nanoscale* **2017**, *9*, 1616–1624.

5. DiDomenico, M.; Wemple, S. H.; Porto, S. P. S.; Bauman, R. P. Raman Spectrum of Single-Domain $BaTiO_3$. *Physical Review* **1968**, *174*, 522–530.

6. Killgore, J. P.; Robins, L.; Collins, L. Electrostatically-blind quantitative piezoresponse force microscopy free of distributed-force artifacts. *Nanoscale Advances* **2022**, *4*, 2036–2045.

⋆⋆⋆
